# Supplementary material for: Unsupervised Pathology Detection: A Deep Dive Into the State of the Art
Source: arXiv:2303.00609 source file (2023-07-29)
Supplement: Supplementary file 1 [file 99-appendix.tex]

\clearpage
\newpage

\section*{Appendix}\label{app}

\subsection{Implementation Details}

We briefly describe hyper-parameter choices and changes we decided to make on the original implementations. For methods that allow for backbone selection, we choose a Wide ResNet-50-2 \cite{wideresnet}. For all experiments we perform 10000 iterations unless stated otherwise. 
\smallskip\newline
\textbf{VAE}\cite{baur2021autoencoders} We adapted a public implementation\footnote{\begin{scriptsize}\url{https://github.com/AntixK/PyTorch-VAE}\end{scriptsize}} and used the architecture from \cite{baur2021autoencoders} as a starting point. We used a held-out subset of the test samples of each dataset to optimize the hyper-parameters in order to achieve the best possible localization performance. Commonly among all modalities, we used a learning rate of 0.0001, Adam optimizer \cite{adam} with no weight-decay, a batch size of 64 and $3 \times 3$ convolutional kernels.
\smallskip\newline
\textbf{f-AnoGAN}\cite{fanogan} We adapted a public PyTorch implementation\footnote{\begin{scriptsize}\url{https://github.com/dbbbbm/f-AnoGAN-PyTorch}\end{scriptsize}} to work for $128 \times 128$ input. We used equal train steps for the Generator and the Discriminator and 30000 steps for training WGANs on the MRI datasets.
\smallskip\newline
\textbf{r-VAE}\cite{gmvae} We used \cite{gmvae} and their provided codebase \footnote{\begin{tiny}\url{https://github.com/yousuhang/Unsupervised-Lesion-Detection-via-Image-Restoration-with-a-Normative-Prior}\end{tiny}} as a guide to implement the restoration algorithm. We found that a learning rate of 1000 worked best for the gradient ascent optimization, as such a high step was necessary for the convergence of the ELBO loss after 500 steps. Restoration was performed on outputs of the already trained VAE models.\smallskip\newline
\textbf{AMCons}\cite{AMCons} We followed the official implementation\footnote{\begin{scriptsize}\url{https://github.com/jusiro/constrained_anomaly_segmentation}\end{scriptsize}}.
\smallskip\newline
\textbf{FAE}\cite{FAE} We followed the official implementation\footnote{\begin{scriptsize}\url{https://github.com/FeliMe/feature-autoencoder}\end{scriptsize}}.
\smallskip\newline
% \textbf{DFR}\cite{DFR} We based our implementation on the official one\footnote{\begin{scriptsize}\url{https://github.com/YoungGod/DFR}\end{scriptsize}}. A higher learning rate of 0.001 is used and a stride of 2 for the mean filter to accommodate for the lower resolution. We re-implemented the Principal Component Analysis algorithm to work with faster PyTorch modules, allowing for a more robust and accurate latent dimension estimation. We tried to implement the method with a Wide ResNet-50-2 with no success, so we used the original backbone choice.
% \smallskip\newline
\textbf{PaDiM}\cite{padim} We followed the unofficial implementation\footnote{\begin{scriptsize}\url{https://github.com/xiahaifeng1995/PaDiM-Anomaly-Detection-Localization-master}\end{scriptsize}}. We used torch.functional.interpolate to upscale the feature maps.
\smallskip\newline
\textbf{CFLOW-AD}\cite{cflow} We followed the official implementation\footnote{\begin{scriptsize}\url{https://github.com/gudovskiy/cflow-ad}\end{scriptsize}}. Originally, the authors use anomalous batch statistics to normalize the likelihood maps. This implies prior knowledge on the test distribution, can affect evaluation given different batch size and sample order, and might also be impractical in real applications. We instead normalize using statistics from a specific validation set batch.
\smallskip\newline
\textbf{RD}\cite{RD} We followed the official implementation\footnote{\begin{scriptsize}\url{https://github.com/hq-deng/RD4AD}\end{scriptsize}}. We used a batch size of 4, which we found to be a more robust choice in our experiments.
\smallskip\newline
\textbf{PII}\cite{pii} We based our implementation on the official one\footnote{\begin{scriptsize}\url{https://github.com/jemtan/PII}\end{scriptsize}}. For MRI, we made sure patches where sampled from and blended on brain pixels only.
\smallskip\newline
\textbf{DAE}\cite{DAE} We followed the official implementation\footnote{\begin{scriptsize}\url{https://github.com/AntanasKascenas/DenoisingAE}\end{scriptsize}}.
\smallskip\newline
\textbf{CCD}\cite{ccd} We followed the official implementation\footnote{\begin{scriptsize}\url{https://github.com/tianyu0207/CCD}\end{scriptsize}} and omitted the local part of the method. We pre-train every backbone for 20000 iterations, except DAE's encoder which was trained with 10000 steps.  We chose permutation as the augmentation and a single layer MLP for the classification task. We choose all the above hyperparameters after testing on many dataset-model combinations. Finally, convergence was not trivial for every encoder. To tackle that, we modified the learning rate and/or the last encoder layers (mostly fully connected ones) of models that required it in order to train properly.
\newline
% \begin{table*}[t]
% \centering
% \caption{Detection and localization results with standard deviation of selected methods on the MRI datasets.}
% \label{tab:main_std}
% \resizebox{\linewidth}{!}{
% \begin{tabular}{lcccccccccccccccccccc}
% \toprule
%  & \multicolumn{4}{c}{\textbf{BraTS-T2}} &  & \multicolumn{4}{c}{\textbf{BraTS-T1}} &  & \multicolumn{4}{c}{\textbf{ATLAS}} &  & \multicolumn{4}{c}{\textbf{DDR}} \\
% \cmidrule(r{4pt}){1-1}\cmidrule{2-5}\cmidrule{7-10}\cmidrule{12-15}\cmidrule{17-20}
% Method & \api & AUROC & \app & \dice &  & \api & AUROC & \app & \dice &  & \api & AUROC & \app & \dice &  & \api & AUROC & \app & \dice & \\
% \cmidrule(r{4pt}){1-1}\cmidrule{2-5}\cmidrule{7-10}\cmidrule{12-15}\cmidrule{17-20}
% VAE & 68$\pm$2 & 73$\pm$1 & 28$\pm$2 & 33$\pm$1 &  & 64$\pm$1 & 70$\pm$1 & 13$\pm$1 & 19$\pm$1 &  & 57$\pm$2 & 76$\pm$1 & 11$\pm$2 & 20$\pm$1 &  & 48$\pm$2 & 48$\pm$1 & 2$\pm$0 & 5$\pm$0 \\
% r-VAE & 75$\pm$0 & 77$\pm$0 & 36$\pm$1 & 40$\pm$1 &  & \\
% \bottomrule
% \end{tabular}}
% \end{table*}

\begin{table*}[t]
\centering
\caption{Detection and localization results with standard deviation of selected methods on the MRI datasets.}
\label{tab:main_std}
\resizebox{\linewidth}{!}{
\begin{tabular}{lccccccccccccccccccc}
\toprule
 & \multicolumn{4}{c}{\textbf{ATLAS}} &  & \multicolumn{4}{c}{\textbf{BraTS-T1}} &  & \multicolumn{4}{c}{\textbf{BraTS-T2}} \\
\cmidrule(r{4pt}){1-1}\cmidrule{2-5}\cmidrule{7-10}\cmidrule{12-15}
Method & \begin{scriptsize}AP\textsubscript{i}\end{scriptsize} & \begin{scriptsize}AUROC\end{scriptsize} & \begin{scriptsize}AP\textsubscript{p}\end{scriptsize} & \begin{scriptsize}$\lceil$Dice$\rceil$ \end{scriptsize}&  & \begin{scriptsize}AP\textsubscript{i}\end{scriptsize} & \begin{scriptsize}AUROC\end{scriptsize} & \begin{scriptsize}AP\textsubscript{p}\end{scriptsize} & \begin{scriptsize}$\lceil$Dice$\rceil$ \end{scriptsize}&  & \begin{scriptsize}AP\textsubscript{i}\end{scriptsize} & \begin{scriptsize}AUROC\end{scriptsize} & \begin{scriptsize}AP\textsubscript{p}\end{scriptsize}& \begin{scriptsize}$\lceil$Dice$\rceil$ \end{scriptsize}\\
\cmidrule(r{4pt}){1-1}\cmidrule{2-5}\cmidrule{7-10}\cmidrule{12-15}
VAE      & 0.57
  \begin{scriptsize}(0.02)\end{scriptsize}                    & 0.76 \begin{scriptsize}(0.01)\end{scriptsize}                    & 0.11 \begin{scriptsize}(0.01)\end{scriptsize}                  & 0.20 \begin{scriptsize}(0.02)\end{scriptsize}   & ~                     & 0.64
  \begin{scriptsize}(0.01)\end{scriptsize}                   & 0.70
  \begin{scriptsize}(0.01)\end{scriptsize}                    & 0.13
  \begin{scriptsize}(0.01)\end{scriptsize}                 & 0.19
  \begin{scriptsize}(0.01)\end{scriptsize}                 & ~                     & 0.68
  \begin{scriptsize}(0.02)\end{scriptsize}                   & 0.73
  \begin{scriptsize}(0.01)\end{scriptsize}                   & 0.28
  \begin{scriptsize}(0.02)\end{scriptsize}                 & 0.33
  \begin{scriptsize}(0.01)\end{scriptsize}                 \\
r-VAE    & 0.60
  \begin{scriptsize}(0.00)\end{scriptsize}                       & 0.78 \begin{scriptsize}(0.00)\end{scriptsize}                      & 0.09 \begin{scriptsize}(0.00)\end{scriptsize}                    & 0.17 \begin{scriptsize}(0.00)\end{scriptsize}   & ~                     & 0.70 \begin{scriptsize}(0.01)\end{scriptsize}                      & 0.76 \begin{scriptsize}(0.00)\end{scriptsize}                       & 0.13 \begin{scriptsize}(0.00)\end{scriptsize}                     & 0.19 \begin{scriptsize}(0.00)\end{scriptsize}                     & ~                     & 0.75 \begin{scriptsize}(0.00)\end{scriptsize}                       & 0.77 \begin{scriptsize}(0.00)\end{scriptsize}                       & 0.36 \begin{scriptsize}(0.01)\end{scriptsize}                   & 0.40 \begin{scriptsize}(0.01)\end{scriptsize}                    \\
f-AnoGAN & 0.26
  \begin{scriptsize}(0.01)\end{scriptsize}                    & 0.46 \begin{scriptsize}(0.04)\end{scriptsize}                    & 0.02 \begin{scriptsize}(0.01)\end{scriptsize}                  & 0.06 \begin{scriptsize}(0.03)\end{scriptsize}  & ~                     & 0.48 \begin{scriptsize}(0.02)\end{scriptsize}                     & 0.53 \begin{scriptsize}(0.02)\end{scriptsize}                     & 0.06 \begin{scriptsize}(0.01)\end{scriptsize}                   & 0.12 \begin{scriptsize}(0.01)\end{scriptsize}                   & ~                     & 0.56 \begin{scriptsize}(0.07)\end{scriptsize}                     & 0.61 \begin{scriptsize}(0.06)\end{scriptsize}                     & 0.15 \begin{scriptsize}(0.04)\end{scriptsize}                   & 0.21 \begin{scriptsize}(0.04)\end{scriptsize}                   \\
AMCons   & 0.32
  \begin{scriptsize}(0.02)\end{scriptsize} & \multicolumn{1}{l}{0.53 \begin{scriptsize}(0.02)\end{scriptsize}} & \multicolumn{1}{l}{0.01 \begin{scriptsize}(0.00)\end{scriptsize}} & 0.03 \begin{scriptsize}(0.00)\end{scriptsize}   & \multicolumn{1}{l}{~} & \multicolumn{1}{l}{0.61 \begin{scriptsize}(0.02)\end{scriptsize}} & \multicolumn{1}{l}{0.64 \begin{scriptsize}(0.02)\end{scriptsize}} & \multicolumn{1}{l}{0.05 \begin{scriptsize}(0.00)\end{scriptsize}} & \multicolumn{1}{l}{0.12 \begin{scriptsize}(0.00)\end{scriptsize}} & \multicolumn{1}{l}{~} & \multicolumn{1}{l}{0.78 \begin{scriptsize}(0.01)\end{scriptsize}} & \multicolumn{1}{l}{0.78 \begin{scriptsize}(0.01)\end{scriptsize}} & \multicolumn{1}{l}{0.35 \begin{scriptsize}(0.00)\end{scriptsize}} & \multicolumn{1}{l}{0.40 \begin{scriptsize}(0.00)\end{scriptsize}}  \\
FAE      & 0.50
  \begin{scriptsize}(0.00)\end{scriptsize}    & 0.73 \begin{scriptsize}(0.00)\end{scriptsize}                       & 0.08 \begin{scriptsize}(0.00)\end{scriptsize}                     & 0.18 \begin{scriptsize}(0.00)\end{scriptsize}   & ~                     & 0.86 \begin{scriptsize}(0.00)\end{scriptsize}                       & 0.85 \begin{scriptsize}(0.00)\end{scriptsize}                       & 0.42 \begin{scriptsize}(0.00)\end{scriptsize}                     & 0.45 \begin{scriptsize}(0.00)\end{scriptsize}                     & ~                     & 0.87 \begin{scriptsize}(0.00)\end{scriptsize}                       & 0.87 \begin{scriptsize}(0.00)\end{scriptsize}                       & 0.51 \begin{scriptsize}(0.00)\end{scriptsize}                     & 0.52 \begin{scriptsize}(0.00)\end{scriptsize}                     \\
% DFR      & 0.37
%   \begin{scriptsize}(0.01)\end{scriptsize} & 0.58 \begin{scriptsize}(0.01)\end{scriptsize}                     & 0.05 \begin{scriptsize}(0.00)\end{scriptsize}                     & 0.12 \begin{scriptsize}(0.00)\end{scriptsize}   & ~                     & 0.58 \begin{scriptsize}(0.01)\end{scriptsize}                     & 0.64 \begin{scriptsize}(0.01)\end{scriptsize}                     & 0.19 \begin{scriptsize}(0.01)\end{scriptsize}                   & 0.27 \begin{scriptsize}(0.01)\end{scriptsize}                   & ~                     & 0.67 \begin{scriptsize}(0.01)\end{scriptsize}                     & 0.69 \begin{scriptsize}(0.01)\end{scriptsize}                     & 0.34 \begin{scriptsize}(0.00)\end{scriptsize}                     & 0.37 \begin{scriptsize}(0.00)\end{scriptsize}                     \\
PaDiM    & 0.34
  \begin{scriptsize}(0.04)\end{scriptsize} & 0.56 \begin{scriptsize}(0.04)\end{scriptsize}                     & 0.05 \begin{scriptsize}(0.00)\end{scriptsize}                     & 0.13 \begin{scriptsize}(0.01)\end{scriptsize} & ~                     & 0.60 \begin{scriptsize}(0.02)\end{scriptsize}                      & 0.65 \begin{scriptsize}(0.02)\end{scriptsize}                     & 0.21 \begin{scriptsize}(0.02)\end{scriptsize}                   & 0.28 \begin{scriptsize}(0.02)\end{scriptsize}                   & ~                     & 0.66 \begin{scriptsize}(0.02)\end{scriptsize}                     & 0.68 \begin{scriptsize}(0.01)\end{scriptsize}                     & 0.34 \begin{scriptsize}(0.02)\end{scriptsize}                   & 0.38 \begin{scriptsize}(0.01)\end{scriptsize}                   \\
CFLOW-AD & 0.40
  \begin{scriptsize}(0.02)\end{scriptsize}  & 0.62 \begin{scriptsize}(0.02)\end{scriptsize}                     & 0.04 \begin{scriptsize}(0.01)\end{scriptsize}                   & 0.10 \begin{scriptsize}(0.02)\end{scriptsize}  & ~                     & 0.65 \begin{scriptsize}(0.06)\end{scriptsize}                     & 0.69 \begin{scriptsize}(0.06)\end{scriptsize}                     & 0.16 \begin{scriptsize}(0.03)\end{scriptsize}                   & 0.24 \begin{scriptsize}(0.04)\end{scriptsize}                   & ~                     & 0.71 \begin{scriptsize}(0.01)\end{scriptsize}                     & 0.72 \begin{scriptsize}(0.01)\end{scriptsize}                     & 0.31 \begin{scriptsize}(0.01)\end{scriptsize}                   & 0.35 \begin{scriptsize}(0.00)\end{scriptsize}                     \\
RD        & 0.55
  \begin{scriptsize}(0.00)\end{scriptsize}   & 0.77 \begin{scriptsize}(0.00)\end{scriptsize}                       & 0.11 \begin{scriptsize}(0.00)\end{scriptsize}                     & 0.22 \begin{scriptsize}(0.00)\end{scriptsize}   & ~                     & 0.81 \begin{scriptsize}(0.01)\end{scriptsize}                     & 0.83 \begin{scriptsize}(0.00)\end{scriptsize}                       & 0.36 \begin{scriptsize}(0.01)\end{scriptsize}                   & 0.42 \begin{scriptsize}(0.01)\end{scriptsize}                   & ~                     & 0.85 \begin{scriptsize}(0.01)\end{scriptsize}                     & 0.85 \begin{scriptsize}(0.01)\end{scriptsize}                     & 0.47 \begin{scriptsize}(0.01)\end{scriptsize}                   & 0.50 \begin{scriptsize}(0.01)\end{scriptsize}                    \\
PII      & 0.37
  \begin{scriptsize}(0.04)\end{scriptsize} & 0.60 \begin{scriptsize}(0.03)\end{scriptsize}                      & 0.03 \begin{scriptsize}(0.00)\end{scriptsize}                     & 0.07 \begin{scriptsize}(0.01)\end{scriptsize} &  ~                     & 0.54 \begin{scriptsize}(0.03)\end{scriptsize}                     & 0.64 \begin{scriptsize}(0.03)\end{scriptsize}                     & 0.13 \begin{scriptsize}(0.01)\end{scriptsize}                   & 0.22 \begin{scriptsize}(0.02)\end{scriptsize}                   & ~                     & 0.57 \begin{scriptsize}(0.07)\end{scriptsize}                     & 0.62 \begin{scriptsize}(0.09)\end{scriptsize}                     & 0.13 \begin{scriptsize}(0.04)\end{scriptsize}                   & 0.22 \begin{scriptsize}(0.05)\end{scriptsize}                   \\
DAE      & 0.44
  \begin{scriptsize}(0.02)\end{scriptsize} & 0.65 \begin{scriptsize}(0.01)\end{scriptsize}                     & 0.05 \begin{scriptsize}(0.01)\end{scriptsize}                   & 0.13 \begin{scriptsize}(0.01)\end{scriptsize} & ~                     & 0.70 \begin{scriptsize}(0.01)\end{scriptsize}                      & 0.74 \begin{scriptsize}(0.01)\end{scriptsize}                     & 0.13 \begin{scriptsize}(0.01)\end{scriptsize}                   & 0.20 \begin{scriptsize}(0.01)\end{scriptsize}                    & ~                     & 0.81 \begin{scriptsize}(0.01)\end{scriptsize}                     & 0.80 \begin{scriptsize}(0.01)\end{scriptsize}                      & 0.47 \begin{scriptsize}(0.02)\end{scriptsize}                   & 0.49 \begin{scriptsize}(0.01)\end{scriptsize}                   \\
Random   & 0.26                                                                                                  & 0.50                                                                                                & 0.01                                                                                              & 0.02                                                                                              &                       & 0.48                                                                                                & 0.50                                                                                                & 0.06                                                                                              & 0.11                                                                                              &                       & 0.48                                                                                                & 0.50                                                                                                & 0.06                                                                                              & 0.11                                                                                              \\
\bottomrule
\end{tabular}}
\end{table*}

\begin{table*}[htb]
\centering
\caption{Detection and localization results with standard deviation of selected methods on the MRI datasets after self-supervised pre-training.}
\label{tab:pretrain_std}
\resizebox{\linewidth}{!}{
\begin{tabular}{lccccccccccccccccccc}
\toprule
 & \multicolumn{4}{c}{\textbf{ATLAS}} &  & \multicolumn{4}{c}{\textbf{BraTS-T1}} &  & \multicolumn{4}{c}{\textbf{BraTS-T2}} \\
\cmidrule(r{4pt}){1-1}\cmidrule{2-5}\cmidrule{7-10}\cmidrule{12-15}
Method & \begin{scriptsize}AP\textsubscript{i}\end{scriptsize} & \begin{scriptsize}AUROC\end{scriptsize} & \begin{scriptsize}AP\textsubscript{p}\end{scriptsize} & \begin{scriptsize}$\lceil$Dice$\rceil$ \end{scriptsize}&  & \begin{scriptsize}AP\textsubscript{i}\end{scriptsize} & \begin{scriptsize}AUROC\end{scriptsize} & \begin{scriptsize}AP\textsubscript{p}\end{scriptsize} & \begin{scriptsize}$\lceil$Dice$\rceil$ \end{scriptsize}&  & \begin{scriptsize}AP\textsubscript{i}\end{scriptsize} & \begin{scriptsize}AUROC\end{scriptsize} & \begin{scriptsize}AP\textsubscript{p}\end{scriptsize}& \begin{scriptsize}$\lceil$Dice$\rceil$ \end{scriptsize}\\
\cmidrule(r{4pt}){1-1}\cmidrule{2-5}\cmidrule{7-10}\cmidrule{12-15}
VAE      & 0.57
  \begin{scriptsize}(0.02)\end{scriptsize} & 0.76
  \begin{scriptsize}(0.01)\end{scriptsize} & 0.11
  \begin{scriptsize}(0.01)\end{scriptsize}                 & 0.20
  \begin{scriptsize}(0.02)\end{scriptsize} &~                     & 0.64
  \begin{scriptsize}(0.01)\end{scriptsize}                   & 0.70
  \begin{scriptsize}(0.01)\end{scriptsize}                    & 0.13
  \begin{scriptsize}(0.01)\end{scriptsize}                 & 0.19
  \begin{scriptsize}(0.01)\end{scriptsize}                 & ~                     & 0.68
  \begin{scriptsize}(0.02)\end{scriptsize}                   & 0.73
  \begin{scriptsize}(0.01)\end{scriptsize}                   & 0.27
  \begin{scriptsize}(0.02)\end{scriptsize}                   & 0.33
  \begin{scriptsize}(0.01)\end{scriptsize}                    \\
r-VAE   &  0.61
  \begin{scriptsize}(0.00)\end{scriptsize}   & 0.79 \begin{scriptsize}(0.00)\end{scriptsize}     & 0.09 \begin{scriptsize}(0.00)\end{scriptsize}                     & 0.17 \begin{scriptsize}(0.00)\end{scriptsize}    & ~                     & 0.70 \begin{scriptsize}(0.01)\end{scriptsize}                      & 0.76 \begin{scriptsize}(0.00)\end{scriptsize}                       & 0.13 \begin{scriptsize}(0.00)\end{scriptsize}                     & 0.19 \begin{scriptsize}(0.00)\end{scriptsize}                     & ~                     & 0.75 \begin{scriptsize}(0.00)\end{scriptsize}                        & 0.77 \begin{scriptsize}(0.00)\end{scriptsize}                        & 0.36 \begin{scriptsize}(0.01)\end{scriptsize}                        & 0.40 \begin{scriptsize}(0.01)\end{scriptsize}                          \\
f-AnoGAN & 0.28
  \begin{scriptsize}(0.01)\end{scriptsize} & 0.5 \begin{scriptsize}(0.03)\end{scriptsize}    & 0.02 \begin{scriptsize}(0.01)\end{scriptsize}                   & 0.04 \begin{scriptsize}(0.02)\end{scriptsize}  &  ~                     & 0.48 \begin{scriptsize}(0.02)\end{scriptsize}                     & 0.53 \begin{scriptsize}(0.02)\end{scriptsize}                     & 0.06 \begin{scriptsize}(0.00)\end{scriptsize}                     & 0.11 \begin{scriptsize}(0.00)\end{scriptsize}                     & ~                     & 0.63 \begin{scriptsize}(0.02)\end{scriptsize}                     & 0.70 \begin{scriptsize}(0.02)\end{scriptsize}                      & 0.15 \begin{scriptsize}(0.01)\end{scriptsize}                     & 0.21 \begin{scriptsize}(0.00)\end{scriptsize}                        \\
AMCons  & 0.31
  \begin{scriptsize}(0.03)\end{scriptsize} & 0.52 \begin{scriptsize}(0.03)\end{scriptsize}   & \multicolumn{1}{l}{0.01 \begin{scriptsize}(0.00)\end{scriptsize}} & 0.03 \begin{scriptsize}(0.00)\end{scriptsize}    & \multicolumn{1}{l}{~} & \multicolumn{1}{l}{0.61 \begin{scriptsize}(0.01)\end{scriptsize}} & \multicolumn{1}{l}{0.64 \begin{scriptsize}(0.02)\end{scriptsize}} & \multicolumn{1}{l}{0.06 \begin{scriptsize}(0.00)\end{scriptsize}} & \multicolumn{1}{l}{0.12 \begin{scriptsize}(0.00)\end{scriptsize}} & \multicolumn{1}{l}{~} & \multicolumn{1}{l}{0.73 \begin{scriptsize}(0.05)\end{scriptsize}} & \multicolumn{1}{l}{0.74 \begin{scriptsize}(0.03)\end{scriptsize}} & \multicolumn{1}{l}{0.27 \begin{scriptsize}(0.07)\end{scriptsize}} & \multicolumn{1}{l}{0.34 \begin{scriptsize}(0.06)\end{scriptsize}}  \\
FAE      & 0.53
  \begin{scriptsize}(0.00)\end{scriptsize}   & 0.75 \begin{scriptsize}(0.00)\end{scriptsize}     & 0.10 \begin{scriptsize}(0.00)\end{scriptsize}                      & 0.21 \begin{scriptsize}(0.00)\end{scriptsize}    & ~                     & 0.85 \begin{scriptsize}(0.00)\end{scriptsize}                       & 0.85 \begin{scriptsize}(0.00)\end{scriptsize}                       & 0.43 \begin{scriptsize}(0.01)\end{scriptsize}                   & 0.46 \begin{scriptsize}(0.00)\end{scriptsize}                     & ~                     & 0.89 \begin{scriptsize}(0.00)\end{scriptsize}                       & 0.88 \begin{scriptsize}(0.00)\end{scriptsize}                       & 0.55 \begin{scriptsize}(0.01)\end{scriptsize}                     & 0.55 \begin{scriptsize}(0.00)\end{scriptsize}                        \\
% DFR       & 0.46
%   \begin{scriptsize}(0.02)\end{scriptsize} & 0.70 \begin{scriptsize}(0.03)\end{scriptsize}    & 0.07 \begin{scriptsize}(0.00)\end{scriptsize}                     & 0.18 \begin{scriptsize}(0.01)\end{scriptsize}  & ~                     & 0.73 \begin{scriptsize}(0.02)\end{scriptsize}                     & 0.77 \begin{scriptsize}(0.01)\end{scriptsize}                     & 0.32 \begin{scriptsize}(0.02)\end{scriptsize}                   & 0.37 \begin{scriptsize}(0.01)\end{scriptsize}                   & ~                     & 0.76 \begin{scriptsize}(0.04)\end{scriptsize}                     & 0.78 \begin{scriptsize}(0.01)\end{scriptsize}                     & 0.46 \begin{scriptsize}(0.03)\end{scriptsize}                     & 0.47 \begin{scriptsize}(0.01)\end{scriptsize}                      \\
PaDiM    & 0.41
  \begin{scriptsize}(0.07)\end{scriptsize} & 0.65 \begin{scriptsize}(0.08)\end{scriptsize}   & 0.07 \begin{scriptsize}(0.01)\end{scriptsize}                   & 0.16 \begin{scriptsize}(0.02)\end{scriptsize}  &  ~                     & 0.74 \begin{scriptsize}(0.04)\end{scriptsize}                     & 0.78 \begin{scriptsize}(0.02)\end{scriptsize}                     & 0.26 \begin{scriptsize}(0.06)\end{scriptsize}                   & 0.32 \begin{scriptsize}(0.04)\end{scriptsize}                   & ~                     & 0.81 \begin{scriptsize}(0.02)\end{scriptsize}                     & 0.81 \begin{scriptsize}(0.02)\end{scriptsize}                     & 0.47 \begin{scriptsize}(0.03)\end{scriptsize}                     & 0.48 \begin{scriptsize}(0.02)\end{scriptsize}                      \\
CFLOW-AD & 0.45
  \begin{scriptsize}(0.02)\end{scriptsize} & 0.68 \begin{scriptsize}(0.02)\end{scriptsize}   & 0.06 \begin{scriptsize}(0.01)\end{scriptsize}                   & 0.14 \begin{scriptsize}(0.02)\end{scriptsize}  & ~                     & 0.76 \begin{scriptsize}(0.03)\end{scriptsize}                     & 0.78 \begin{scriptsize}(0.03)\end{scriptsize}                     & 0.24 \begin{scriptsize}(0.03)\end{scriptsize}                   & 0.30 \begin{scriptsize}(0.03)\end{scriptsize}                    & ~                     & 0.79 \begin{scriptsize}(0.00)\end{scriptsize}                       & 0.80 \begin{scriptsize}(0.00)\end{scriptsize}                        & 0.31 \begin{scriptsize}(0.03)\end{scriptsize}                     & 0.38 \begin{scriptsize}(0.02)\end{scriptsize}                      \\
RD       & 0.42
  \begin{scriptsize}(0.13)\end{scriptsize} & 0.64 \begin{scriptsize}(0.12)\end{scriptsize}   & 0.05 \begin{scriptsize}(0.06)\end{scriptsize}                   & 0.09 \begin{scriptsize}(0.10)\end{scriptsize}   & ~                     & 0.74 \begin{scriptsize}(0.03)\end{scriptsize}                     & 0.78 \begin{scriptsize}(0.02)\end{scriptsize}                     & 0.28 \begin{scriptsize}(0.02)\end{scriptsize}                   & 0.35 \begin{scriptsize}(0.02)\end{scriptsize}                   & ~                     & 0.84 \begin{scriptsize}(0.02)\end{scriptsize}                     & 0.85 \begin{scriptsize}(0.02)\end{scriptsize}                     & 0.39 \begin{scriptsize}(0.05)\end{scriptsize}                     & 0.44 \begin{scriptsize}(0.04)\end{scriptsize}                      \\
PII       & 0.32
  \begin{scriptsize}(0.02)\end{scriptsize} & 0.52 \begin{scriptsize}(0.05)\end{scriptsize}   & 0.02 \begin{scriptsize}(0.01)\end{scriptsize}                   & 0.05 \begin{scriptsize}(0.02)\end{scriptsize}  & ~                     & 0.46 \begin{scriptsize}(0.07)\end{scriptsize}                     & 0.50\begin{scriptsize}(0.10)\end{scriptsize}                       & 0.07 \begin{scriptsize}(0.03)\end{scriptsize}                   & 0.14 \begin{scriptsize}(0.03)\end{scriptsize}                   & ~                     & 0.60 \begin{scriptsize}(0.15)\end{scriptsize}                      & 0.66 \begin{scriptsize}(0.17)\end{scriptsize}                     & 0.11 \begin{scriptsize}(0.04)\end{scriptsize}                     & 0.19 \begin{scriptsize}(0.06)\end{scriptsize}                      \\
DAE      & 0.47
  \begin{scriptsize}(0.04)\end{scriptsize} & 0.68 \begin{scriptsize}(0.03)\end{scriptsize}   & 0.07 \begin{scriptsize}(0.02)\end{scriptsize}                   & 0.15 \begin{scriptsize}(0.02)\end{scriptsize}  & ~                     & 0.71 \begin{scriptsize}(0.03)\end{scriptsize}                     & 0.75 \begin{scriptsize}(0.01)\end{scriptsize}                     & 0.14 \begin{scriptsize}(0.02)\end{scriptsize}                   & 0.20 \begin{scriptsize}(0.01)\end{scriptsize}                    & ~                     & 0.81 \begin{scriptsize}(0.01)\end{scriptsize}                     & 0.81 \begin{scriptsize}(0.01)\end{scriptsize}                     & 0.48 \begin{scriptsize}(0.05)\end{scriptsize}                     & 0.50 \begin{scriptsize}(0.02)\end{scriptsize}                       \\
Random   & 0.26                                                                                                  & 0.50                                                                                                & 0.01                                                                                              & 0.02                                                                                              &                       & 0.48                                                                                                & 0.50                                                                                                & 0.06                                                                                              & 0.11                                                                                              &                       & 0.48                                                                                                & 0.50                                                                                                & 0.06                                                                                                & 0.11                                                                                                 \\
\bottomrule
\end{tabular}}
\end{table*}

\begin{table*}[t]
\centering
\caption{Detection and localization results with standard deviation of selected methods on the RF and CXR datasets.}
\label{tab:main_std_2}
\resizebox{\linewidth}{!}{
\begin{tabular}{lccccccccccccc} 
\toprule
 & \multicolumn{4}{c}{\textbf{DDR}}& \multicolumn{1}{l}{} & \multicolumn{2}{c}{\textbf{CheXpert - Pleural Effusion}}& & \multicolumn{2}{c}{\textbf{\textbf{CheXpert - Opacity}}}& \multicolumn{1}{c}{} & \multicolumn{2}{c}{\textbf{CheXpert - Enlarged Card.}} \\ 
\cmidrule(r{4pt}){1-1}\cmidrule{2-5}\cmidrule{7-8}\cmidrule{10-11}\cmidrule{13-14}
Method & \begin{scriptsize}AP\textsubscript{i}\end{scriptsize} & \begin{scriptsize}AUROC\end{scriptsize} & \begin{scriptsize}AP\textsubscript{p}\end{scriptsize} & \begin{scriptsize}$\lceil$Dice$\rceil$\end{scriptsize}&& \begin{scriptsize}AP\textsubscript{i}\end{scriptsize} & \begin{scriptsize}AUROC\end{scriptsize} & & \begin{scriptsize}AP\textsubscript{i}\end{scriptsize} & \begin{scriptsize}AUROC\end{scriptsize} && \begin{scriptsize}AP\textsubscript{i}\end{scriptsize} & \begin{scriptsize}AUROC\end{scriptsize} \\ 
\cmidrule(lr){1-1}\cmidrule{2-5}\cmidrule{7-8}\cmidrule{10-11}\cmidrule{13-14}
VAE& 0.48
\begin{scriptsize}(0.02)\end{scriptsize} & 0.48
\begin{scriptsize}(0.01)\end{scriptsize} & 0.02
\begin{scriptsize}(0.00)\end{scriptsize} & 0.05
\begin{scriptsize}(0.00)\end{scriptsize} & ~& 0.55
\begin{scriptsize}(0.00)\end{scriptsize} & 0.57
\begin{scriptsize}(0.01)\end{scriptsize} & ~ & 0.51
\begin{scriptsize}(0.00)\end{scriptsize} & 0.54
\begin{scriptsize}(0.01)\end{scriptsize} & ~& 0.56
\begin{scriptsize}(0.00)\end{scriptsize} & 0.56
\begin{scriptsize}(0.01)\end{scriptsize}\\
r-VAE& 0.51
\begin{scriptsize}(0.01)\end{scriptsize} & 0.50 \begin{scriptsize}(0.01)\end{scriptsize}& 0.03 \begin{scriptsize}(0.01)\end{scriptsize} & 0.08 \begin{scriptsize}(0.02)\end{scriptsize} & ~& 0.52
\begin{scriptsize}(0.00)\end{scriptsize} & 0.57 \begin{scriptsize}(0.00)\end{scriptsize} & ~ & 0.47 \begin{scriptsize}(0.00)\end{scriptsize} & 0.5 \begin{scriptsize}(0.01)\end{scriptsize}& ~& 0.52 \begin{scriptsize}(0.02)\end{scriptsize} & 0.56 \begin{scriptsize}(0.02)\end{scriptsize}\\
f-AnoGAN & 0.44
\begin{scriptsize}(0.02)\end{scriptsize} & 0.45 \begin{scriptsize}(0.01)\end{scriptsize} & 0.01 \begin{scriptsize}(0.00)\end{scriptsize} & 0.01 \begin{scriptsize}(0.00)\end{scriptsize} & ~& 0.59
\begin{scriptsize}(0.00)\end{scriptsize} & 0.61 \begin{scriptsize}(0.00)\end{scriptsize} & ~ & 0.49 \begin{scriptsize}(0.01)\end{scriptsize} & 0.51 \begin{scriptsize}(0.02)\end{scriptsize} & ~& 0.57 \begin{scriptsize}(0.00)\end{scriptsize} & 0.59 \begin{scriptsize}(0.00)\end{scriptsize}\\
AMCons & 0.49
\begin{scriptsize}(0.00)\end{scriptsize} & 0.49 \begin{scriptsize}(0.00)\end{scriptsize} & 0.004 \begin{scriptsize}(0.00)\end{scriptsize} & 0.01 \begin{scriptsize}(0.00)\end{scriptsize} & ~& 0.39
\begin{scriptsize}(0.01)\end{scriptsize} & 0.31 \begin{scriptsize}(0.03)\end{scriptsize} & ~ & 0.49 \begin{scriptsize}(0.02)\end{scriptsize} & 0.48 \begin{scriptsize}(0.03)\end{scriptsize} & ~& 0.41 \begin{scriptsize}(0.01)\end{scriptsize} & 0.37 \begin{scriptsize}(0.02)\end{scriptsize}\\
FAE& 0.64
\begin{scriptsize}(0.00)\end{scriptsize} & 0.63 \begin{scriptsize}(0.01)\end{scriptsize} & 0.07 \begin{scriptsize}(0.00)\end{scriptsize} & 0.15 \begin{scriptsize}(0.00)\end{scriptsize} & ~& 0.73
\begin{scriptsize}(0.00)\end{scriptsize} & 0.77 \begin{scriptsize}(0.00)\end{scriptsize} & ~ & 0.57 \begin{scriptsize}(0.00)\end{scriptsize} & 0.61 \begin{scriptsize}(0.00)\end{scriptsize} & ~& 0.63 \begin{scriptsize}(0.00)\end{scriptsize} & 0.66 \begin{scriptsize}(0.00)\end{scriptsize}\\
% DFR& 0.56
% \begin{scriptsize}(0.00)\end{scriptsize} & 0.53 \begin{scriptsize}(0.01)\end{scriptsize} & 0.06 \begin{scriptsize}(0.00)\end{scriptsize} & 0.14 \begin{scriptsize}(0.00)\end{scriptsize} & ~& 0.56
% \begin{scriptsize}(0.00)\end{scriptsize} & 0.60 \begin{scriptsize}(0.00)\end{scriptsize}& ~ & 0.47 \begin{scriptsize}(0.00)\end{scriptsize} & 0.49 \begin{scriptsize}(0.00)\end{scriptsize} & ~& 0.57 \begin{scriptsize}(0.00)\end{scriptsize} & 0.60 \begin{scriptsize}(0.00)\end{scriptsize} \\
PaDiM& 0.55
\begin{scriptsize}(0.02)\end{scriptsize} & 0.55 \begin{scriptsize}(0.02)\end{scriptsize} & 0.02 \begin{scriptsize}(0.00)\end{scriptsize} & 0.07 \begin{scriptsize}(0.01)\end{scriptsize} & ~& 0.61
\begin{scriptsize}(0.00)\end{scriptsize} & 0.66 \begin{scriptsize}(0.00)\end{scriptsize} & ~ & 0.50 \begin{scriptsize}(0.00)\end{scriptsize}& 0.52 \begin{scriptsize}(0.00)\end{scriptsize} & ~& 0.60 \begin{scriptsize}(0.00)\end{scriptsize}& 0.63 \begin{scriptsize}(0.00)\end{scriptsize}\\
CFLOW-AD & 0.51
\begin{scriptsize}(0.01)\end{scriptsize} & 0.51 \begin{scriptsize}(0.02)\end{scriptsize} & 0.03 \begin{scriptsize}(0.00)\end{scriptsize} & 0.08 \begin{scriptsize}(0.00)\end{scriptsize} & ~& 0.67
\begin{scriptsize}(0.00)\end{scriptsize} & 0.73 \begin{scriptsize}(0.00)\end{scriptsize} & ~ & 0.52 \begin{scriptsize}(0.00)\end{scriptsize} & 0.54 \begin{scriptsize}(0.00)\end{scriptsize} & ~& 0.62 \begin{scriptsize}(0.00)\end{scriptsize} & 0.66 \begin{scriptsize}(0.00)\end{scriptsize}\\
RD & 0.66
\begin{scriptsize}(0.00)\end{scriptsize} & 0.64 \begin{scriptsize}(0.00)\end{scriptsize} & 0.10 \begin{scriptsize}(0.00)\end{scriptsize}& 0.19 \begin{scriptsize}(0.00)\end{scriptsize} & ~& 0.65
\begin{scriptsize}(0.00)\end{scriptsize} & 0.71 \begin{scriptsize}(0.00)\end{scriptsize} & ~ & 0.54 \begin{scriptsize}(0.00)\end{scriptsize} & 0.58 \begin{scriptsize}(0.00)\end{scriptsize} & ~& 0.61 \begin{scriptsize}(0.00)\end{scriptsize} & 0.63 \begin{scriptsize}(0.00)\end{scriptsize}\\
PII& 0.62
\begin{scriptsize}(0.03)\end{scriptsize} & 0.63 \begin{scriptsize}(0.02)\end{scriptsize} & 0.01 \begin{scriptsize}(0.00)\end{scriptsize} & 0.01 \begin{scriptsize}(0.00)\end{scriptsize} & ~& 0.64
\begin{scriptsize}(0.05)\end{scriptsize} & 0.65 \begin{scriptsize}(0.04)\end{scriptsize} & ~ & 0.53 \begin{scriptsize}(0.03)\end{scriptsize} & 0.54 \begin{scriptsize}(0.04)\end{scriptsize} & ~& 0.56 \begin{scriptsize}(0.03)\end{scriptsize} & 0.56 \begin{scriptsize}(0.04)\end{scriptsize}\\
DAE& 0.54
\begin{scriptsize}(0.07)\end{scriptsize} & 0.55 \begin{scriptsize}(0.09)\end{scriptsize} & 0.01 \begin{scriptsize}(0.00)\end{scriptsize} & 0.03 \begin{scriptsize}(0.01)\end{scriptsize} & ~& 0.63
\begin{scriptsize}(0.00)\end{scriptsize} & 0.65 \begin{scriptsize}(0.00)\end{scriptsize} & ~ & 0.52 \begin{scriptsize}(0.01)\end{scriptsize} & 0.55 \begin{scriptsize}(0.01)\end{scriptsize} & ~& 0.58 \begin{scriptsize}(0.01)\end{scriptsize} & 0.60 \begin{scriptsize}(0.01)\end{scriptsize} \\
Random & 0.26& 0.50& 0.004 & 0.01&& 0.50& 0.50& & 0.50& 0.50&& 0.50& 0.50 \\
\bottomrule
\end{tabular}}
\end{table*}

\begin{table*}[htb]
\centering
\caption{Detection and localization results with standard deviation of selected methods on the RF and CXR datasets after self-supervised pre-training.}
\label{tab:pretrain_std_2}
\resizebox{\linewidth}{!}{
\begin{tabular}{lccccccccccccc} 
\toprule
 & \multicolumn{4}{c}{\textbf{DDR}}& \multicolumn{1}{l}{} & \multicolumn{2}{c}{\textbf{CheXpert - Pleural Effusion}}& & \multicolumn{2}{c}{\textbf{\textbf{CheXpert - Opacity}}}& \multicolumn{1}{c}{} & \multicolumn{2}{c}{\textbf{CheXpert - Enlarged Card.}} \\ 
\cmidrule(r{4pt}){1-1}\cmidrule{2-5}\cmidrule{7-8}\cmidrule{10-11}\cmidrule{13-14}
Method & \begin{scriptsize}AP\textsubscript{i}\end{scriptsize} & \begin{scriptsize}AUROC\end{scriptsize} & \begin{scriptsize}AP\textsubscript{p}\end{scriptsize} & \begin{scriptsize}$\lceil$Dice$\rceil$\end{scriptsize}&& \begin{scriptsize}AP\textsubscript{i}\end{scriptsize} & \begin{scriptsize}AUROC\end{scriptsize} & & \begin{scriptsize}AP\textsubscript{i}\end{scriptsize} & \begin{scriptsize}AUROC\end{scriptsize} && \begin{scriptsize}AP\textsubscript{i}\end{scriptsize} & \begin{scriptsize}AUROC\end{scriptsize}\\ 
\cmidrule(lr){1-1}\cmidrule{2-5}\cmidrule{7-8}\cmidrule{10-11}\cmidrule{13-14}
VAE& 0.48
\begin{scriptsize}(0.01)\end{scriptsize} & 0.48
\begin{scriptsize}(0.02)\end{scriptsize} & 0.02
\begin{scriptsize}(0.00)\end{scriptsize} & 0.05
\begin{scriptsize}(0.00)\end{scriptsize} & ~& 0.56
\begin{scriptsize}(0.00)\end{scriptsize} & 0.58
\begin{scriptsize}(0.00)\end{scriptsize} & ~& 0.52
\begin{scriptsize}(0.00)\end{scriptsize} & 0.54
\begin{scriptsize}(0.00)\end{scriptsize} & ~& 0.56
\begin{scriptsize}(0.00)\end{scriptsize} & 0.57
\begin{scriptsize}(0.00)\end{scriptsize}\\
r-VAE& 0.49
\begin{scriptsize}(0.04)\end{scriptsize} & 0.48 \begin{scriptsize}(0.03)\end{scriptsize} & 0.02 \begin{scriptsize}(0.02)\end{scriptsize} & 0.09 \begin{scriptsize}(0.00)\end{scriptsize} & ~& 0.52
\begin{scriptsize}(0.00)\end{scriptsize} & 0.57 \begin{scriptsize}(0.01)\end{scriptsize} & ~& 0.47 \begin{scriptsize}(0.00)\end{scriptsize} & 0.49 \begin{scriptsize}(0.01)\end{scriptsize} & ~& 0.52 \begin{scriptsize}(0.02)\end{scriptsize} & 0.56 \begin{scriptsize}(0.02)\end{scriptsize}\\
f-AnoGAN & 0.41
\begin{scriptsize}(0.01)\end{scriptsize} & 0.42 \begin{scriptsize}(0.01)\end{scriptsize} & 0.01 \begin{scriptsize}(0.00)\end{scriptsize} & 0.01 \begin{scriptsize}(0.00)\end{scriptsize} & ~& 0.60
\begin{scriptsize}(0.01)\end{scriptsize}& 0.62 \begin{scriptsize}(0.00)\end{scriptsize} & ~& 0.50   \begin{scriptsize}(0.00)\end{scriptsize}& 0.52 \begin{scriptsize}(0.00)\end{scriptsize} & ~& 0.58 \begin{scriptsize}(0.01)\end{scriptsize} & 0.60 \begin{scriptsize}(0.01)\end{scriptsize} \\
AMCons & 0.49
\begin{scriptsize}(0.02)\end{scriptsize} & 0.50 \begin{scriptsize}(0.00)\end{scriptsize}& 0.004 \begin{scriptsize}(0.00)\end{scriptsize} & 0.01 \begin{scriptsize}(0.00)\end{scriptsize} & ~& 0.43
\begin{scriptsize}(0.05)\end{scriptsize} & 0.40 \begin{scriptsize}(0.08)\end{scriptsize}& ~& 0.50 \begin{scriptsize}(0.01)\end{scriptsize}& 0.52 \begin{scriptsize}(0.01)\end{scriptsize} & ~& 0.45 \begin{scriptsize}(0.04)\end{scriptsize} & 0.43 \begin{scriptsize}(0.06)\end{scriptsize}\\
FAE& 0.55
\begin{scriptsize}(0.02)\end{scriptsize} & 0.57 \begin{scriptsize}(0.01)\end{scriptsize} & 0.03 \begin{scriptsize}(0.00)\end{scriptsize} & 0.08 \begin{scriptsize}(0.00)\end{scriptsize} & ~& 0.74
\begin{scriptsize}(0.00)\end{scriptsize} & 0.78 \begin{scriptsize}(0.00)\end{scriptsize} & ~& 0.55 \begin{scriptsize}(0.00)\end{scriptsize} & 0.58 \begin{scriptsize}(0.00)\end{scriptsize} & ~& 0.65 \begin{scriptsize}(0.00)\end{scriptsize} & 0.68 \begin{scriptsize}(0.00)\end{scriptsize}\\
% DFR& 0.53
% \begin{scriptsize}(0.00)\end{scriptsize} & 0.50 \begin{scriptsize}(0.00)\end{scriptsize}& 0.03 \begin{scriptsize}(0.00)\end{scriptsize} & 0.08 \begin{scriptsize}(0.01)\end{scriptsize} & ~& 0.51
% \begin{scriptsize}(0.01)\end{scriptsize} & 0.52 \begin{scriptsize}(0.01)\end{scriptsize} & ~~ & 0.45 \begin{scriptsize}(0.01)\end{scriptsize} & 0.45 \begin{scriptsize}(0.01)\end{scriptsize} & ~& 0.53 \begin{scriptsize}(0.01)\end{scriptsize} & 0.54 \begin{scriptsize}(0.01)\end{scriptsize}\\
PaDiM& 0.54
\begin{scriptsize}(0.02)\end{scriptsize} & 0.54 \begin{scriptsize}(0.01)\end{scriptsize} & 0.02 \begin{scriptsize}(0.00)\end{scriptsize} & 0.05 \begin{scriptsize}(0.00)\end{scriptsize} & ~& 0.59
\begin{scriptsize}(0.01)\end{scriptsize} & 0.63 \begin{scriptsize}(0.01)\end{scriptsize} & ~& 0.48 \begin{scriptsize}(0.00)\end{scriptsize} & 0.49 \begin{scriptsize}(0.01)\end{scriptsize} & ~& 0.58 \begin{scriptsize}(0.00)\end{scriptsize} & 0.60 \begin{scriptsize}(0.01)\end{scriptsize} \\
CFLOW-AD & 0.53
\begin{scriptsize}(0.01)\end{scriptsize} & 0.54 \begin{scriptsize}(0.01)\end{scriptsize} & 0.02 \begin{scriptsize}(0.00)\end{scriptsize} & 0.07 \begin{scriptsize}(0.01)\end{scriptsize} & ~& 0.58
\begin{scriptsize}(0.01)\end{scriptsize} & 0.62 \begin{scriptsize}(0.01)\end{scriptsize} & ~& 0.47 \begin{scriptsize}(0.01)\end{scriptsize} & 0.48 \begin{scriptsize}(0.03)\end{scriptsize} & ~& 0.58 \begin{scriptsize}(0.00)\end{scriptsize} & 0.60 \begin{scriptsize}(0.01)\end{scriptsize} \\
RD & 0.53
\begin{scriptsize}(0.03)\end{scriptsize} & 0.54 \begin{scriptsize}(0.02)\end{scriptsize} & 0.04 \begin{scriptsize}(0.00)\end{scriptsize} & 0.09 \begin{scriptsize}(0.01)\end{scriptsize} & ~& 0.66
\begin{scriptsize}(0.02)\end{scriptsize} & 0.69 \begin{scriptsize}(0.02)\end{scriptsize} & ~& 0.55 \begin{scriptsize}(0.01)\end{scriptsize} & 0.58 \begin{scriptsize}(0.01)\end{scriptsize} & ~& 0.61 \begin{scriptsize}(0.01)\end{scriptsize} & 0.62 \begin{scriptsize}(0.01)\end{scriptsize}\\
PII& 0.60
\begin{scriptsize}(0.04)\end{scriptsize}& 0.60 \begin{scriptsize}(0.05)\end{scriptsize}& 0.01 \begin{scriptsize}(0.00)\end{scriptsize} & 0.04 \begin{scriptsize}(0.01)\end{scriptsize} & ~& 0.65
\begin{scriptsize}(0.03)\end{scriptsize} & 0.66 \begin{scriptsize}(0.03)\end{scriptsize} & ~& 0.52 \begin{scriptsize}(0.03)\end{scriptsize} & 0.53 \begin{scriptsize}(0.03)\end{scriptsize} & ~& 0.58 \begin{scriptsize}(0.02)\end{scriptsize} & 0.59 \begin{scriptsize}(0.02)\end{scriptsize}\\
DAE& 0.59
\begin{scriptsize}(0.05)\end{scriptsize} & 0.60 \begin{scriptsize}(0.04)\end{scriptsize}& 0.01 \begin{scriptsize}(0.00)\end{scriptsize} & 0.03 \begin{scriptsize}(0.01)\end{scriptsize} & ~& 0.62
\begin{scriptsize}(0.01)\end{scriptsize} & 0.64 \begin{scriptsize}(0.00)\end{scriptsize} & ~& 0.52 \begin{scriptsize}(0.01)\end{scriptsize} & 0.54 \begin{scriptsize}(0.01)\end{scriptsize} & ~& 0.58 \begin{scriptsize}(0.01)\end{scriptsize} & 0.60 \begin{scriptsize}(0.01)\end{scriptsize} \\
Random & 0.26& 0.50 & 0.004 & 0.01&& 0.50 & 0.50 && 0.50 & 0.50 && 0.50 & 0.50  \\
\bottomrule

\end{tabular}}
\end{table*}
\begin{figure*}[htbp]
\centerline{\includegraphics[width=0.7\linewidth]{figures/Picture0.png}}
\caption{Highest and lowest scored Pleural Effusion samples of negative (first row) and positive (second row) cases.}
\label{fig:effusion_scores}
\end{figure*}
